# Supplementary material for: Resonance profiles of valley polarization in single-layer MoS$_2$ and MoSe$_2$
Source: arXiv:1801.09497 ancillary file (2018-11-05)
Supplement: Supplementary file 1 [file Supplemental-Material-for-Resonance-profiles-of-valley-polarization-in-single-layer-MoS2-and-MoSe2.pdf]

This article has been published at Physical Review Letters: Phys. Rev. Lett. 121, 167401 (2018).

# Supplemental Material for Resonance profiles of valley polarization in single-layer $MoS_2$ and $MoSe_2$

Hans Tornatzky* and Anne-Marie Kaulitz
*Institut für Festkörperphysik, Technische Universität Berlin, Hardenbergstr. 36, 10623 Berlin, Germany*

Janina Maultzsch
*Institut für Festkörperphysik, Technische Universität Berlin, Hardenbergstr. 36, 10623 Berlin, Germany and Department Physik, Friedrich-Alexander-Universität Erlangen-Nürnberg, Staudtstr. 7, 91058 Erlangen, Germany*

(Dated: November 5, 2018)

## COMPARISON OF DOP $\rho$ VALUES WITH THE LITERATURE

In Fig. S 1 we show our values of the degree of polarization (DOP) $\rho$ of "series 1" $MoS_2$ presented in the main text compared to the values of Ref. [1] and the references within [1], namely [2–5]. They mostly fall well in line with our data.

The work of Mak *et al.* [2] contains a comparison of the circularly polarized photoluminescence (PL) emission of single-layer $MoS_2$ on $SiO_2$ and on h-BN substrate. We have performed a fit of the spectra in Ref. [2] to obtain the intensity and the spectral position of the emission. From this we determined the DOP $\rho$ and the excess energy $\Delta E$. In the spectra of $MoS_2$ on $SiO_2$, the signal-to-noise ratio and the contribution from Raman lines lead to a larger fitting error than in the case of the h-BN substrate.

We have performed the same procedure to obtain the neutral and charged exciton DOP $\rho$ for the spectra presented by Cao *et al.* [3].

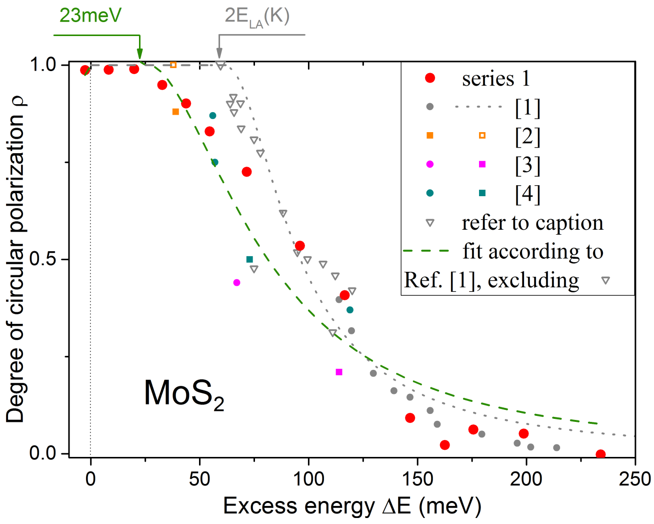


FIG. S 1: Comparison of DOP values measured in our experiments and given in the literature. Circles / squares depict the DOP $\rho$ calculated from the emission originated from the exciton / trion. The value obtained for $MoS_2$ on h-BN ($SiO_2$) from Ref. [2] is depicted as an open (filled) square. Open triangles depict the values of Refs. [2–5] as given in Ref. [1].

TABLE S I: Extracted excess energies $\Delta E$ and degrees of polarization $\rho$ from Refs. [2–4].

| $\Delta E$ (meV) | DOP $\rho$ | remark | | | Ref. |
|---|---|---|---|---|---|
| 38 | 0.98 | $T =$ 14 K | trion | h-BN | [2] |
| 39 | 0.88 | $T =$ 14 K | trion | $SiO_2$ | |
| 114 | 0.21 | $T =$ 83 K | trion | $SiO_2$ | [3] |
| 67 | 0.44 | $T =$ 83 K | exciton | | |
| 73 | 0.50 | $T =$ 4 K | trion | $SiO_2$ | [4] |
| 56 | 0.87 | $T =$ 4 K | exciton | | |
| 57 | 0.75 | $T =$ 125 K | | | |
| 119 | 0.37 | $T =$ 300 K | | | |

In the work of Sallen and co-workers [4], a temperature series of the circular polarization is presented. For three temperatures (4K, 125 K, and 300 K), the circularly resolved spectra are given, of which we extract the DOP $\rho$ and emission energies. Further values could potentially be extracted from the temperature series plot of the circular polarization[7] considering the Varshni equation, however, were omitted here.

The last reference used by the authors of Ref. [1] is another temperature series performed by Zeng *et al.* [5]. In this article no circularly resolved PL spectra are shown, precluding the above process. Here, the polarization coefficient is differently defined as $P = \pm I(\sigma_\pm)/I_{\text{tot}}$. Therefore, we did not consider the data of Ref. [5].

The values of $\rho$ extracted from Refs. [2–4] as described above are summarized in Tab. S I and plotted in Fig. S 1.

Fitting our data and the values of Refs. [1–4] with the model given in Ref. [1], we obtain the curve plotted in Fig. S 1 with a dashed green line. The obtained energy onset of the decline given by the fit is $\hbar\omega_q = 23\,\text{meV}$, different than the value reported in Ref. [1].

We further include in Fig. S 1 the values of Refs. [2–5] (open, grey triangles) as plotted and used to fit the phonon model (dashed grey line) by the authors of Ref. [1].

## EXCITATION-POWER DEPENDENCE OF THE PL OF $MOS_2$

An excitation-power series of the linearly polarized PL has been recorded to exclude laser-induced sample heating. In Fig. S 2, data of the neutral exciton and trion emission of the "series 1" $MoS_2$ sample are shown (the star corresponds to the experiments shown in the main paper). The numbers next to the symbols indicate the measurement order showing that for the first measurements with excitation power below $\approx 350\,\mu W$ (measurements #1, #2, star) solely the neutral exciton emission at constant energy was observed. By increasing the laser power to $\approx 500\,\mu W$, laser-induced changes gain importance and a 4 meV up-shift of the exciton peak as well as the emergence of the trion peak are observed (Fig. S 2). The measurements after the observation of this energy shift (i.e. #4 – #10) show no significant spectral shift up to $555\,\mu W$. Only the measurement #7 (1 mW) exhibits a slight redshift of about 1 meV.

Regarding the apparent shift of the measurement #3 at $387\,\mu W$ compared to the preceding low power measurements, we suggest that it is due to the emerging trion emission. These changes, however, are too small to fit an additional peak for the trion to the acquired data. As the subsequent measurements around $400\,\mu W$ show no exciton shift, we exclude laser-induced sample heating as the source of the shift.

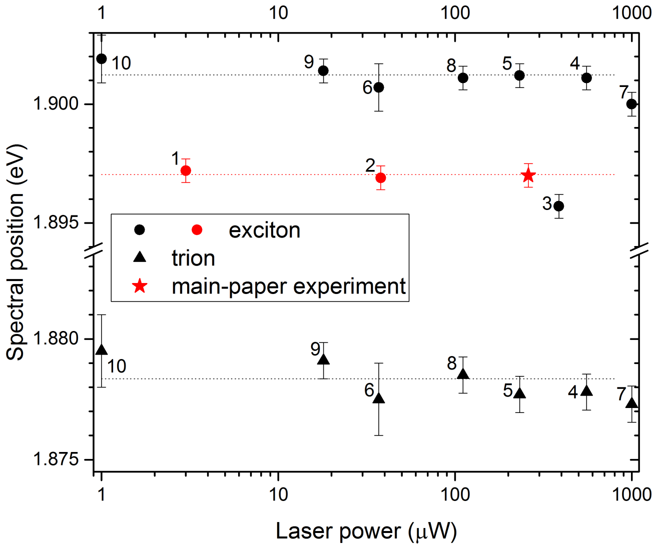


FIG. S 2: Power series of the "series 1" $MoS_2$ sample under the measurement conditions as in the experiments of the main text. Data points corresponding to measurements before and after the emergence of the trion are color coded for better distinction. The exciton spectral position corresponding to the experiments shown in the main paper is included (star). Horizontal lines depict average values, excluding measurements 3 and 7.

As our PL spectra presented in the main text show no shift or broadening compared to the measurements #1 and #2, we are certain that the sample was not subject to laser-induced changes or heating.

## RESONANCES OF THE PHOTOLUMINESCENCE INTENSITIES

Figure S 3 depicts the circularly resolved photoluminescence intensity of the $A$ exciton emission as a function of the excess energy $\Delta E$ for the "series 1" $MoS_2$. The intensity is determined by the area under the Gaussian curve of the fitted peak. With increasing excess energy $\Delta E$ up to $\approx 50$ meV, a reduction of the intensity of the co-polarized emission can be observed. At higher excess energies, the intensity is relatively constant. For the counter-polarized emission one observes an increase of the intensity, starting at zero for $\Delta E = 0$ meV excess energy. Above about 150 meV, it remains roughly constant at about the same value as the co-polarized emission, resulting in the degree of polarization (DOP) $\rho$ converging to $\rho = 0$. We speculate that the reduced emission intensity for the co-polarization at higher excess energies is due to the reduced absorption, when leaving the resonance. This is supported by the potential agreement of the trend of the intensity with the shape of the PL emission.

We argue that the accordance of the equality of co-

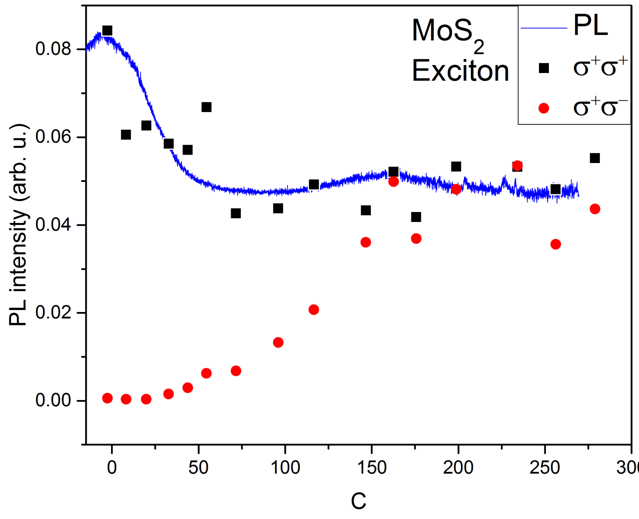


FIG. S 3: Photoluminescence intensity of the $A$ exciton emission of $MoS_2$ as a function of the excess energy. A PL spectrum has been included as i) a guidance for the energy scaling and ii) to visualize the potential accordance with the trend of the co-polarized intensities.

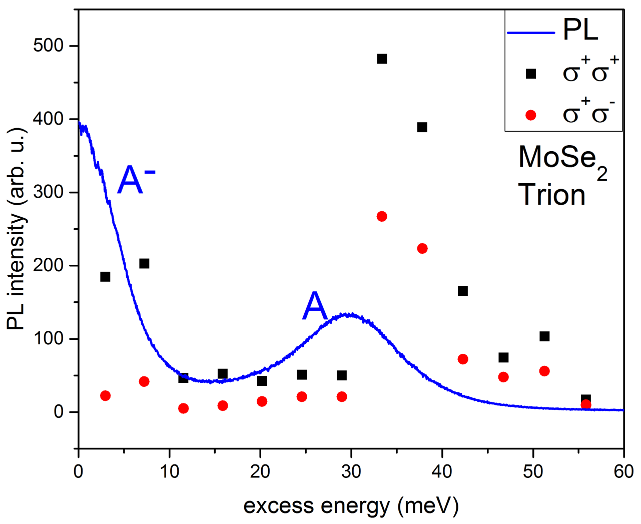


FIG. S 4: Photoluminescence intensity of the and $A^-$ trion emission of $MoSe_2$ as a function of the excess energy. A PL spectrum has been included as a guidance for the energy scaling.

and counter-polarized emission intensity at the valence-band spin-orbit splitting might only be a coincidence, as "series 2" $MoS_2$ sample shows a decay of the DOP $\rho$ at lower excess energies (see Fig. 3 in the main text). Furthermore, if the data of $MoS_2$ and $MoSe_2$ are interpreted in the same picture, one finds that the decline of the counter-polarized emission of $MoSe_2$ (i.e. $\rho$) is only at very low excess energies (see Fig. 3 in the main text), while the valence band splitting occurs at even higher energies than in $MoS_2$.

For $MoSe_2$ (Fig. S 4), we observe strong enhancement of the trion emission at energies around the neutral exciton energy. This stems from the strong absorption and subsequent relaxation into the trion state. The degree of polarization, however, does not drastically change around this energy (see Fig. 3 in the main text), from which we conclude that the degree of polarization of the trion emission is not affected by the additional absorption and relaxation channel.

Note that each pair of co- and counter-polarized measurement (i.e. pair of data points in Figs. S 3 and S 4) was taken at a different spatial position for experimental reasons. Therefore, slight changes in the dielectric environment of the measured spot can lead to strong differences of the PL intensity and thereby result in a significant but unknown error.

## SAMPLES

Figure S 5 depicts optical microscope images of our $MoS_2$ and $MoSe_2$ flakes together with their respective Raman spectra, providing evidence for single layer flakes.

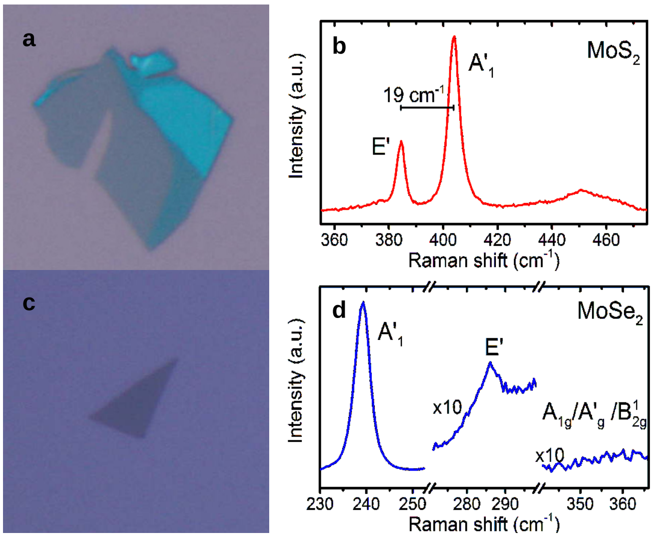


FIG. S 5: a), c) Optical microscope images of used $MoS_2$ (series 1) and $MoSe_2$ flakes; images depict an area of $20 \times 20\,\mu m^2$. b), d) Raman spectra of the $MoS_2$ and $MoSe_2$ flakes with 532 nm excitation. The SL nature is proven by the Raman shift difference of the $A_1'$ and E$'$ for $MoS_2$ and by the observation of the $A_1'$ mode at $\omega = 239\,\mathrm{cm}^{-1}$ and the absence of the few layer/bulk $A_{1g}/A_1'/B_{2g}^1$ mode [6] for $MoSe_2$.

* Electronic address: ht07@physik.tu-berlin.de


[1] G. Kioseoglou, A. T. Hanbicki, M. Currie, A. L. Friedman, and B. T. Jonker, Sci. Rep. **6**, 25041 (2016).

[2] K. F. Mak, K. He, J. Shan, and T. F. Heinz, Nat. Nanotechnol. **7**, 494 (2012).

[3] T. Cao, G. Wang, W. Han, H. Ye, C. Zhu, J. Shi, Q. Niu, P. Tan, E. Wang, B. Liu, et al., Nat. Commun. **3**, 887 (2012).

[4] G. Sallen, L. Bouet, X. Marie, G. Wang, C. R. Zhu, W. P. Han, Y. Lu, P. H. Tan, T. Amand, B. L. Liu, et al., Phys. Rev. B **86**, 081301 (2012).

[5] H. Zeng, J. Dai, W. Yao, D. Xiao, and X. Cui, Nat. Nanotechnol. **7**, 490 (2012).

[6] N. Scheuschner, R. Gillen, M. Staiger, and J. Maultzsch, Phys. Rev. B **91**, 235409 (2015).

[7] In Ref. [4] no definition of the circular polarization percentage is given.
